# Supplementary material for: Three Jahn-Teller states of matter in the spin-crossover system Mn(taa)
Source: arXiv:1912.07770 source file (2020-05-02)
Supplement: Supplementary file 1 [file Mn-taa-prl-suppl.pdf]

# Supplemental materials of: three Jahn-Teller states of matter in spin-crossover system Mn(taa)

Jie-Xiang Yu,[1] Dian-Teng Chen,[1] Jie Gu,[1] Jia Chen,[1] Jun Jiang,[1] Long Zhang,[1] Yue Yu,[1] Xiao-Guang Zhang,[1] Vivien Zapf,[2] and Hai-Ping Cheng[1]

[1] *Department of Physics, Center for Molecular Magnetic Quantum Materials and Quantum Theory Project, University of Florida, Gainesville, Florida 32611, USA*

[2] *National High Magnetic Field Lab (NHMFL), Los Alamos National Lab (LANL), Los Alamos NM 87545, USA*

## I. MONTE CARLO SIMULATIONS

We performed Metropolis Monte-Carlo simulations [1] based on the microscopic Hamiltonian described in the main text. A Markov chain of both electronic-lattice configurations and vibration number contributions of on-site phonon modes was generated. Periodic boundary conditions were applied to a cubic lattice with total of 16384 sites in a unit. Averages over $5.12 \times 10^5$ ensembles for each site were performed at each temperature during both cooling and heating processes from 1 K to 150 K. Subsequently we computed thermal averages of the total energy $E$, occupation number of the HS $\rho_{\mathrm{HS}}$ and the HS ($q = z$) $\rho_{\mathrm{HS-qz}}$ states, the $z$ component of polarization $P_z$ and the nearest neighbor correlation $\langle P^{'}_{z,i} P^{'}_{z,j} \rangle$ of $P_z$, and we also extracted the corresponding thermal fluctuation quantities, the specific heat $c_v = (k_B \beta^2/V)\left(\langle E^2\rangle - \langle E\rangle^2\right)$, the standard deviation of occupation $\delta\rho = \sqrt{\left(\langle\rho^2\rangle - \langle\rho\rangle^2\right)/N}$, electric susceptibility $\chi_e = \varepsilon_r - 1 = (\beta/V\varepsilon_0)\left(\langle P_z^2\rangle - \langle P_z\rangle^2\right)$, and the standard deviation of the correlation $\delta\langle P^{'}_{z,i} P^{'}_{z,j}\rangle = \sqrt{\left(\langle (P^{'}_{z,i} P^{'}_{z,j})^2\rangle - \langle P^{'}_{z,i} P^{'}_{z,j}\rangle^2\right)/N}$.

## II. FIRST-PRINCIPLES CALCULATIONS

The parameters in the Hamiltonian were calculated from first-principles calculations within the framework of density functional theory using the projector augmented wave pseudopotential [2, 3] as implemented in VASP [4, 5]. The generalized gradient approximation (GGA) of Perdew, Burke, and Ernzerhof (PBE) [6] was used for the exchange-correlation energy and the Hubbard $U$ method [7] ($U = 2.5 \sim 4.0\,\mathrm{eV}$, $J = 0.9\,\mathrm{eV}$) was applied on the Mn-($3d$) orbitals. An energy cutoff of 600 eV for the plane-wave expansion was used.

Total energy calculations were performed on both single molecule structures and bulk phases. For single molecule structures, a periodic cubic lattice with a lattice constant of 20.00 Å was used for both LS and HS states to keep the molecules sufficiently separated by the vacuum space. For bulk structures, lattice constants of the cubic unit cell containing 16 Mn(taa) molecules were taken from experimental measurements [8], 19.96 Å for LS and 20.10 Å for HS, respectively. Atomic positions were optimized until the force on each atom was less than 1 meV/Å. Vibration modes of the single molecule structure were obtained using the finite displacement method [9] implemented in the Phonopy package [10].

## III. CONSTRAINED RPA CALCULATION FOR ON-SITE COULOMB INTERACTION

The on-site Coulomb interaction strength can be estimated from first principles using the constrained Random Phase Approximation (cRPA) method [11, 12]. The idea is to calculate the RPA particle-hole polarization with the constraint of a pre-defined exclusion window (e.g. the $d$-like bands around the Fermi level), excluding the polarization originating from the exclusion window. The on-site screened Coulomb interaction is then determined from the constrained RPA particle-hole polarization and the bare Coulomb interaction. The RPA polarization can be calculated from the Kohn-Sham susceptibility, which is solely based on the DFT ground state. In practice, considering 100 empty states above the Fermi level should give a good estimation of the Coulomb interaction $U$. We have an implementation of cRPA within the FP-LAPW method [13, 14]. In the current calculation, we excluded the five $d$-like bands of the Mn

atom and included 100 empty bands. The on-site $U$-matrices are:

$$U_{mm'} = \begin{pmatrix} 3.16 & 2.74 & 2.66 & 2.74 & 2.97 \\ 2.74 & 3.16 & 2.95 & 2.74 & 2.80 \\ 2.66 & 2.95 & 3.28 & 2.77 & 2.54 \\ 2.74 & 2.74 & 2.77 & 3.16 & 2.80 \\ 2.97 & 2.80 & 2.54 & 2.80 & 3.28 \end{pmatrix}$$

$$J_{mm'} = \begin{pmatrix} 3.16 & 0.42 & 0.50 & 0.42 & 0.23 \\ 0.42 & 3.16 & 0.27 & 0.42 & 0.44 \\ 0.50 & 0.27 & 3.28 & 0.27 & 0.51 \\ 0.42 & 0.42 & 0.27 & 3.16 & 0.44 \\ 0.23 & 0.44 & 0.51 & 0.44 & 3.28 \end{pmatrix}$$

The diagonal elements of $U_{mm'}$ (or $J_{mm'}$) are the intra-orbital Coulomb interaction $U$ (average value: 3.21 eV). The off-diagonal elements of $U_{mm'}$ are inter-orbital Coulomb interaction $U'$ (average value: 2.77 eV). The off-diagonal elements of $J_{mm'}$ are the inter-orbital exchange interaction $J$ (average value: 0.39 eV).

## IV. SOME MONTE-CARLO RESULTS

### A. Discussion of inter-molecular strain interaction

Under $A_{hh} = A_{hl} = 0$ (Fig. S1), no peaks are identified in specific heat curves and the spin states gradually change from the LS to the HS as temperature increases without phase transition. It indicates that the strain interaction induces the spin-crossover phase transition.

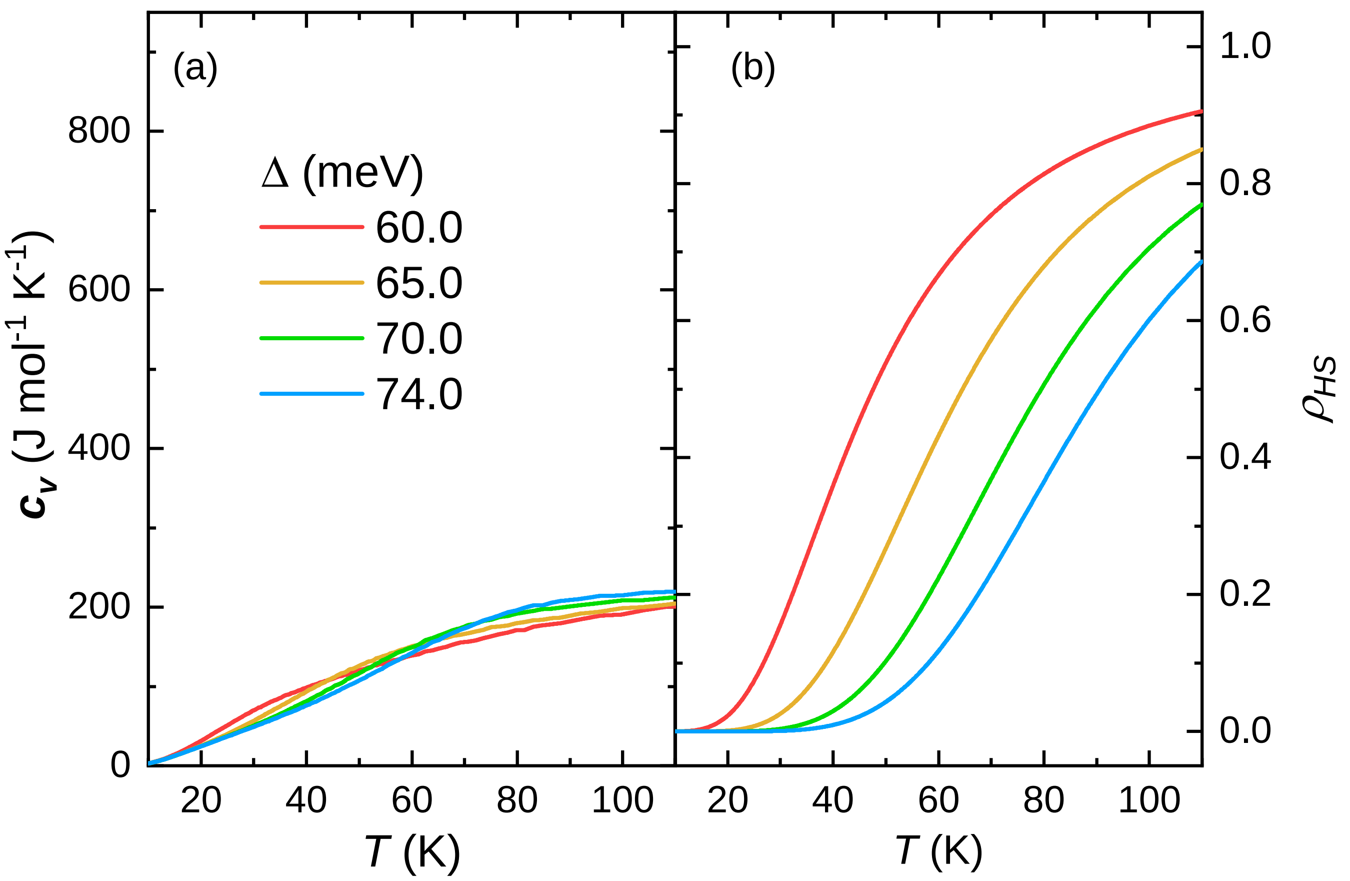


**Fig** S1: Without strain interaction ($A_{hh} = A_{hl} = 0$), the thermal averages of (a) specific heat $c_v$ and (b) population $\rho_{\text{HS}}$ as a function of temperature under zero magnetic field. $D = 0.3$ meV. There is no difference between annealing and heating results.

$A_{hh}$ is the coefficient of the HS-HS strain interaction. We perform simulations under a HS only system with various $A_{hh}$. The results are shown in Fig. S2. A phase transition is identified and the phase transition temperature is strongly dependent on $A_{hh}$. This phase transition corresponds to ordering/disordering of JT distortions.

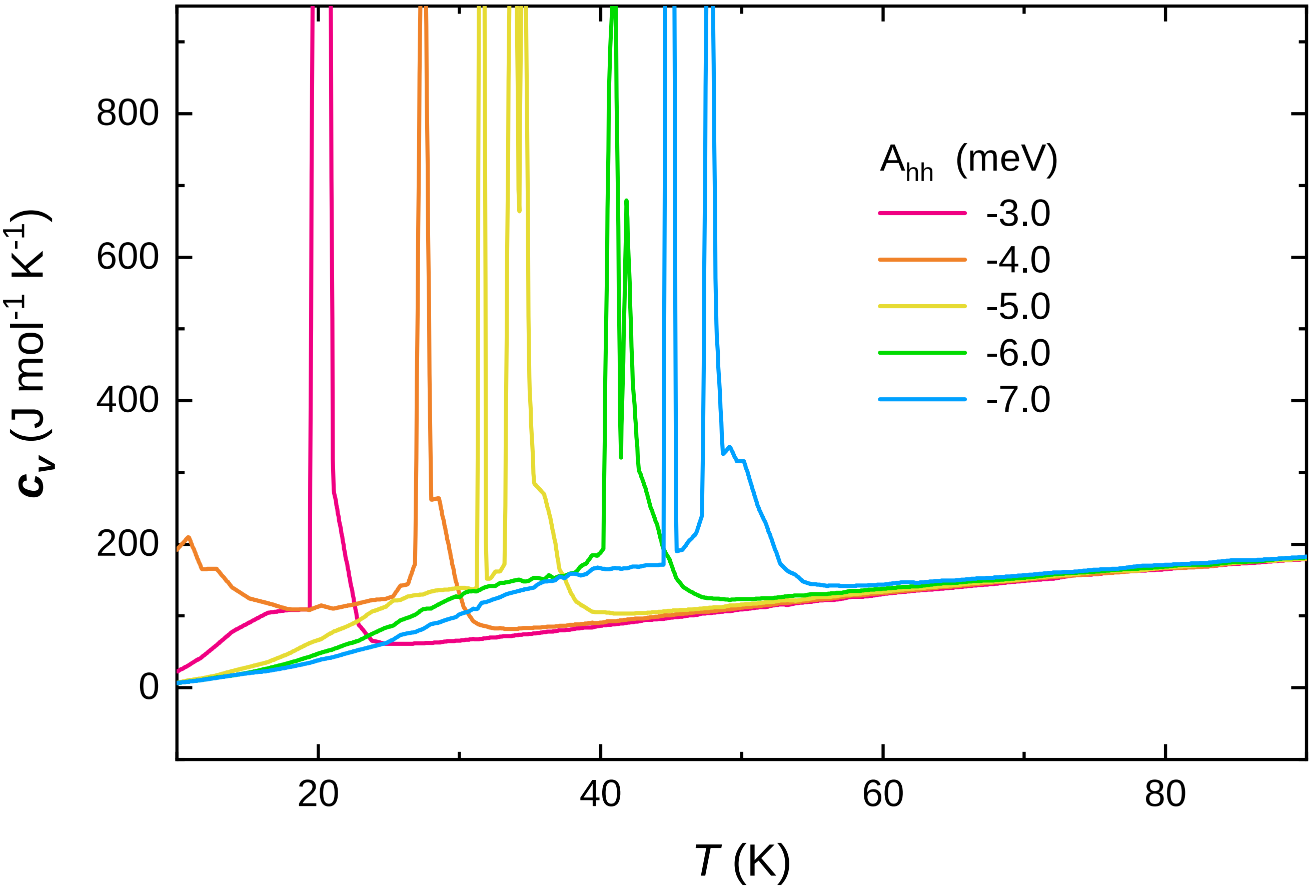


**Fig** S2: In a HS only system, The thermal averages of specific heat $c_v$ as a function of temperature under zero magnetic field. $D = 0.3$ meV There is no difference between annealing and heating results.

$A_{hl}$ is the coefficient of the LS-HS strain interaction. We perform non-magnetic-field simulations with various $A_{hl}$. As a result shown in Fig. S3, $A_{hl}$ controls the size of the hysteresis-like loop during annealing and heating process.

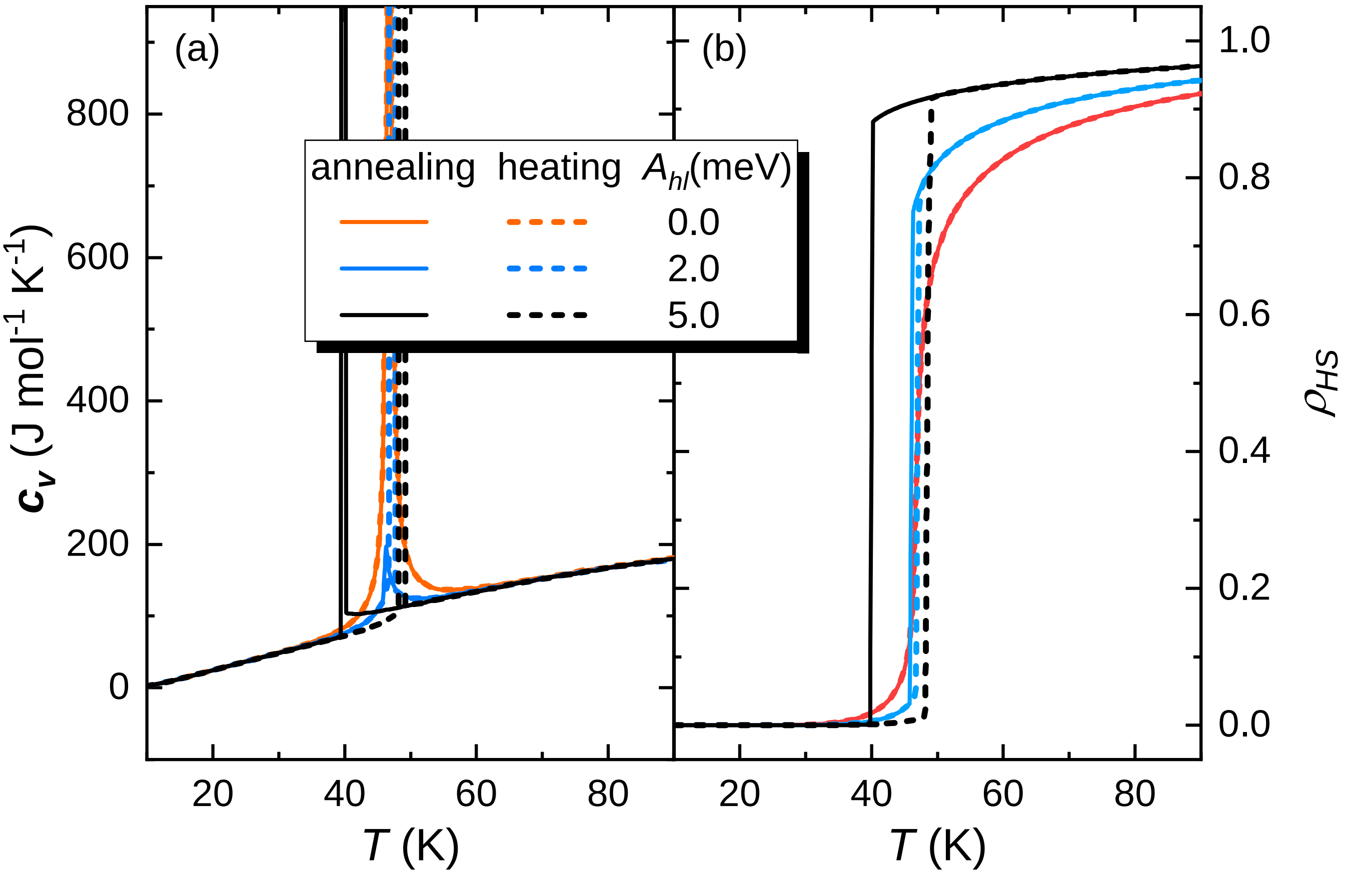


**Fig** S3: With various $A_{hl}$, the thermal averages of (a) specific heat $c_v$ and (b) population $\rho_{\mathrm{HS}}$ as a function of temperature under zero magnetic field. $\Delta = 74.0$ meV, $A_{hh} = 5.0$ meV and $D = 0.3$ meV. Solid and dashed lines correspond to annealing and heating results respectively.

### B. Fluctuation under zero magnetic field

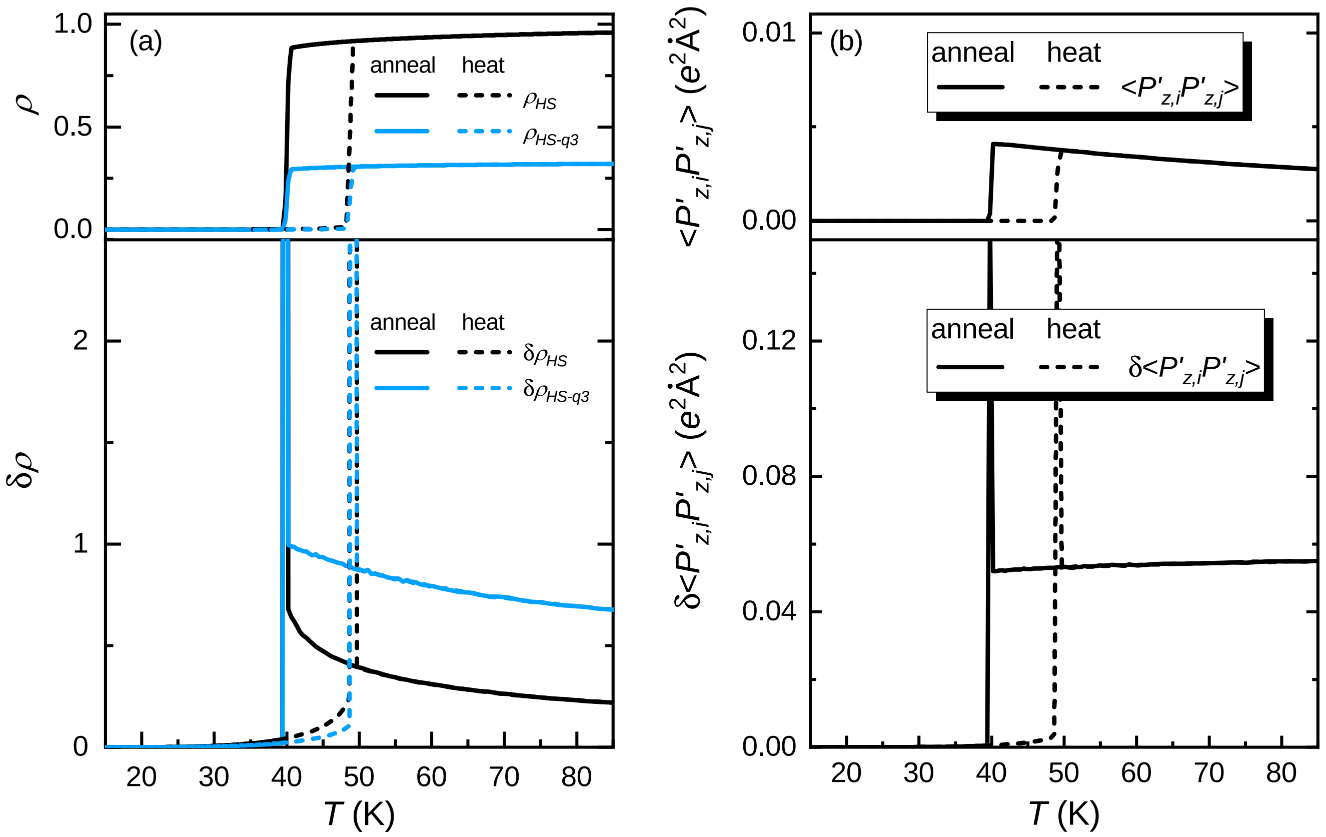


**Fig** S4: The thermal averages (upper panel) and the corresponding standard deviations (lower panel) of (a) population $\rho_{\mathrm{HS}}$ and subpopulation $\rho_{\mathrm{HS}-qz}$ and (b) $\langle P^{'}_{z,i}P^{'}_{z,j}\rangle$ of $P_z$ as a function of temperature under zero magnetic field. Solid and dashed lines refer to annealing and heating processes.

### C. Temperature and magnetic field dependent results with various Δ

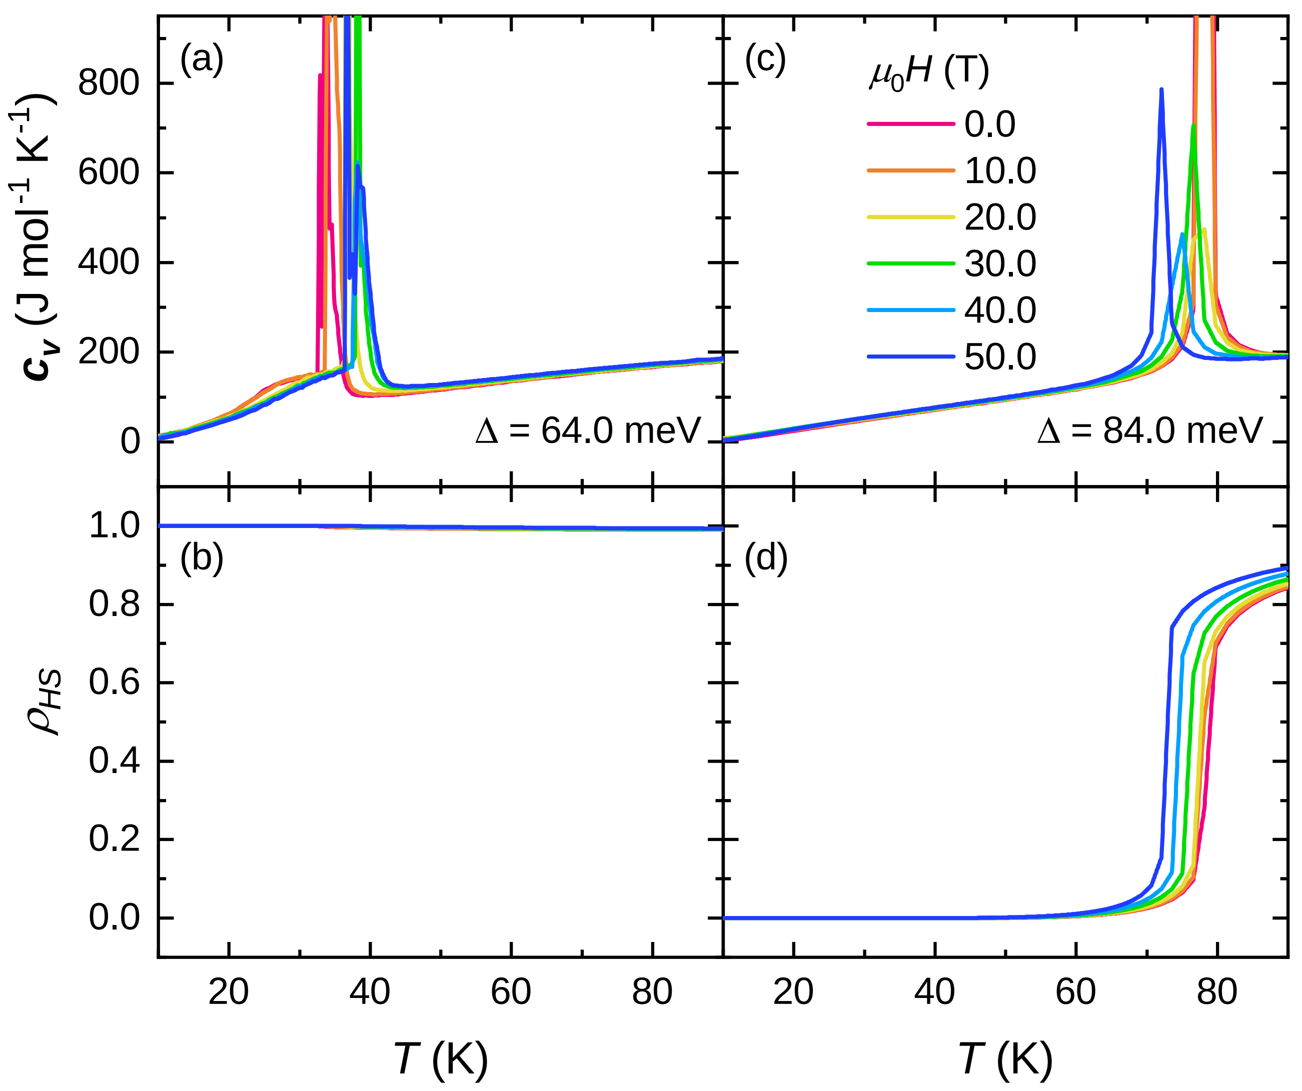


**Fig** S5: With various magnetic fields, (upper) specific heat $c_v$ and (lower) population $\rho_{\mathrm{HS}}$ as a function of temperature under (left) $\Delta = 64.0$ meV and (right) $\Delta = 84.0$ meV.

### D. $\rho_{\mathrm{HS}-qz}$ phase diagram depending on temperature and magnetic field

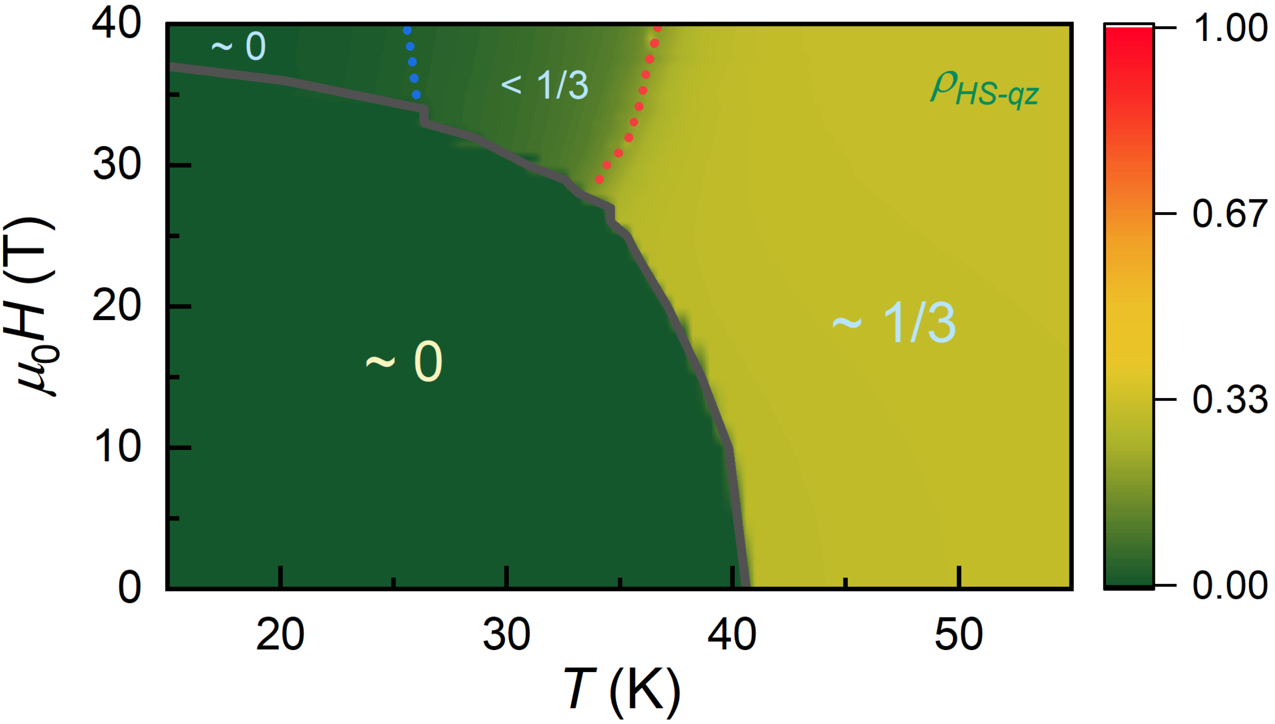


**Fig** S6: The population under annealing of the HS ($q = z$) state $\rho_{\mathrm{HS}-qz}$ as a function of temperature and magnetic field, showing phase boundaries. The magnitude of $\rho_{\mathrm{HS}-qz}$ at each phase is labeled.


[1] N. Metropolis and S. Ulam, J. Am. Stat. Assoc. **44**, 335 (1949).
[2] P. E. Blöchl, Phys. Rev. B **50**, 17953 (1994).
[3] G. Kresse and D. Joubert, Phys. Rev. B **59**, 1758 (1999).
[4] G. Kresse and J. Furthmüller, Comput. Mater. Sci. **6**, 15 (1996).
[5] G. Kresse and J. Furthmüller, Phys. Rev. B **54**, 11169 (1996).
[6] J. P. Perdew, K. Burke, and M. Ernzerhof, Phys. Rev. Lett. **77**, 3865 (1996), .
[7] A. I. Liechtenstein, V. I. Anisimov, and J. Zaanen, Phys. Rev. B **52**, R5467 (1995).
[8] P. Guionneau, M. Marchivie, Y. Garcia, J. A. K. Howard, and D. Chasseau, Phys. Rev. B **72**, 214408 (2005).
[9] K. Parlinski, Z. Q. Li, and Y. Kawazoe, Phys. Rev. Lett. **78**, 4063 (1997).
[10] A. Togo and I. Tanaka, Scr. Mater. **108**, 1 (2015).
[11] F. Aryasetiawan, M. Imada, A. Georges, G. Kotliar, S. Biermann, and A. I. Lichtenstein, Phys. Rev. B **70**, 195104 (2004).
[12] F. Aryasetiawan, K. Karlsson, O. Jepsen, and U. Schönberger, Phys. Rev. B **74**, 125106 (2006).
[13] A. Kozhevnikov, A. G. Eguiluz, and T. C. Schulthess, in *2010 ACM/IEEE International Conference for High Performance Computing, Networking, Storage and Analysis* (IEEE, 2010).
[14] L. Zhang, P. Staar, A. Kozhevnikov, Y.-P. Wang, J. Trinastic, T. Schulthess, and H.-P. Cheng, Phys. Rev. B **100** (2019).
